# Supplementary material for: Spin-orbit driven Peierls transition and possible exotic superconductivity in CsW$_{2}$O$_{6}$
Source: arXiv:1606.02403 source file (2017-01-09)
Supplement: Supplementary file 1 [file SM.pdf]

# Supplemental materials for Spin-orbit driven Peierls transition and possible exotic superconductivity in $CsW_2O_6$

Sergey V. Streltsov,[1,2,*] Igor I. Mazin,[3] Rolf Heid,[4] and Klaus-Peter Bohnen[4]

[1] *M.N. Miheev Institute of Metal Physics of Ural Branch of Russian Academy of Sciences, 620137, Ekaterinburg, Russia*
[2] *Ural Federal University, Mira St. 19, 620002 Ekaterinburg, Russia*
[3] *Code 6393, Naval Research Laboratory, Washington, DC 20375, USA*
[4] *Institue for Solid State Physics, Karlsruhe Institute of Technology (KIT), D-76021 Karlsruhe, Germany*

(Dated: November 29, 2016)

PACS numbers: 75.20.Ck,71.27.+a

## I. EXPERIMENTAL LT STRUCTURE

The crystal structure proposed by Hirai et al[1] for low-T phase consists of zigzag chains with shortened W-W bonds (3.598 Å), see Fig. 1 (left), propagating along the cubic $[1,1,0]$ direction (orthorhombic $b$). This structure can be also visualized as a network of tetramerized linear W chains running along the cubic $[1,0,1]$ and $[0,1,1]$ directions, as shown in Fig. 1 (right). This tetramerization, however, does not open the band gap as seen in Fig. 2 even if the spin-orbit coupling (SOC) or Hubbard correlations are taken into account. Indeed, given 4 electrons per unit cell, and accounting for the Kramer degeneracy, we observe that the gap can be opened only between the second (cyan in Fig. 2) and the third (black) bands. That would require lifting the bottom of the third band at Γ above the top of the second band (at R) by at least 0.3 eV. No meaningful manipulation with this electronic structure or atomic positions can possibly open the gap, unless the unit cell size is increased.

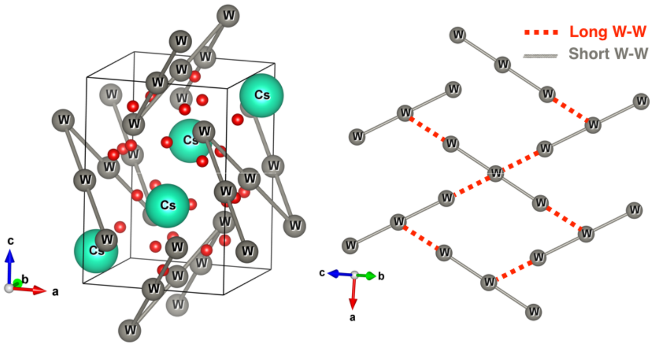


Figure 1: Crystal structure obtained in Ref. [1] for T=110 K (low-T phase). In right panel the W-W network is shown.

*Electronic address: streltsov@imp.uran.ru

## II. PHONON CALCULATIONS

Phonon calculations for the fcc structure of $CsW_2O_6$ were performed within a mixed-basis pseudopotential framework [2, 3] using density-functional perturbation theory (DFPT) [4, 5]. Norm-conserving pseudopotentials including non-linear core corrections were constructed from all-electron relativistic atom calculations according to the scheme of Vanderbilt [6]. The spin-orbit coupling is incorporated within the pseudopotential approach [7, 8] and is treated fully self-consistently.[9]) Calculations were performed within the generalized-gradient approximation.[10] Plane waves up to a kinetic energy of 24 Ry were augmented with local functions of $p$ and $d$ type at the Cs sites, and $s$, $p$, and $d$ types at W, and $s$ and $p$ at the O sites. This choice of the basis set guaranteed sufficient convergence of electronic and phononic properties. Brillouin zone summations were performed on a fcc $8\times8\times8$ $k$-point mesh in combination with the standard

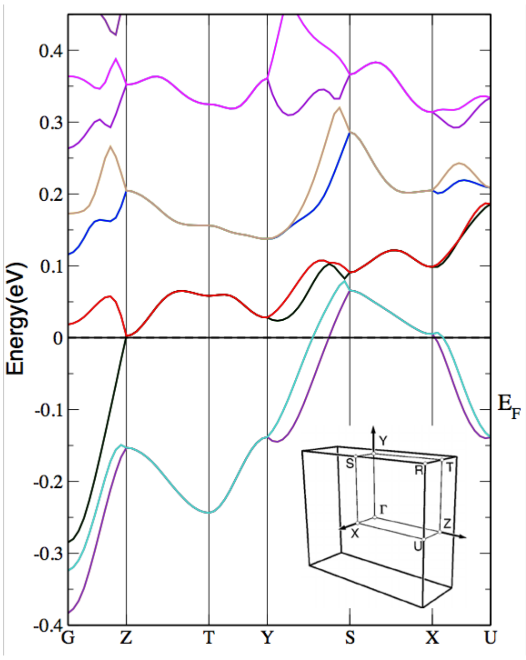


Figure 2: The band structure obtained for the LT structure of Ref. [1] in the GGA+SOC calculations (Wien2k).

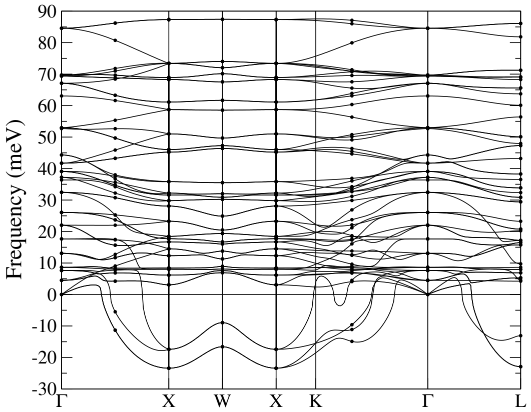


Figure 3: Phonon spectrum as obtained in the GGA+SOC calculations for the optimized high temperature structure.

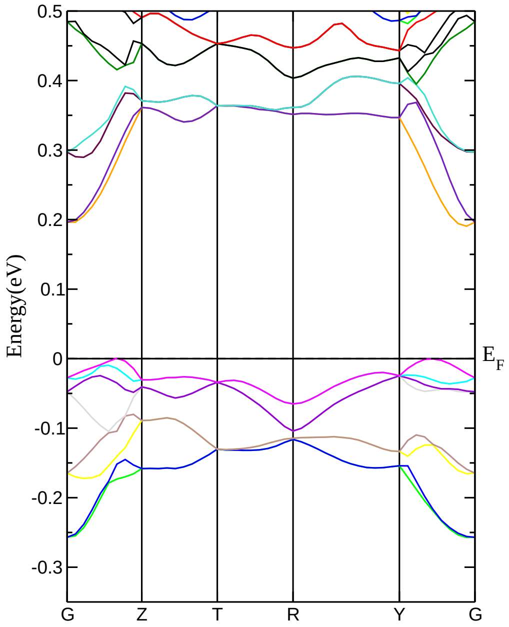


Figure 4: The band structure obtained for optimized low-T structure in the GGA+SOC calculations (Wien2k).

smearing technique [11] employing a Gaussian broadening of 0.1 eV. Dynamical matrices were determined via DFPT on a simple cubic 2×2×2 $q$-point mesh (32 points in the full Brillouin zone), and were then interpolated for arbitrary $q$ points using a standard Fourier technique. Resulting phonon spectrum is shown in Fig. 3.

## III. GGA+SOC OPTIMIZED STRUCTURE

As it is explained in the main part of the paper we optimized (in VASP) the crystal structure of $CsW_2O_6$

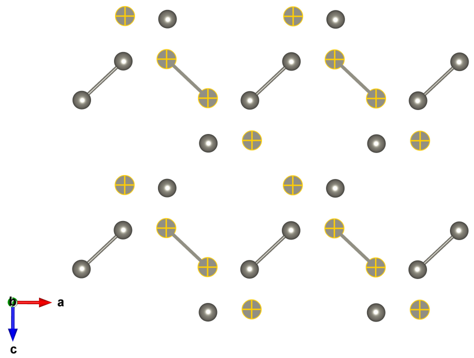


Figure 5: The W lattice in the GGA+SOC optimized $P2_12_12_1$ structure. W ions, which belong to two different $ac$ planes are shown by different colours. No tetramerization is found in the $b$ direction.

using combination of eigenvectors of two unstable phonon modes as an input. Resulting crystal structure of the $P4_132$ symmetry still gives metallic ground state, while further decrease of the symmetry down to $P2_12_12_1$ opens a gap. Corresponding band structure is shown in Fig. 4. $CsW_2O_6$ is a band insulator with both valence and conduction bands formed mostly by W 5$d$ states. There are 16 W ions in the unit cell (4 classes with 4 equivalent W in each class) in the optimized $P2_12_12_1$ structure and eight $d$ (each W is nominally 5.5+, i.e. $d^{0.5}$) electrons occupy all the valence bands.

The crystal structure is characterized by tetramerized W-W chains running in two orthogonal directions in two different $ac$ plane, see Fig. 5. The cif-file of optimized crystal structure is enclosed to this SM.


[1] D. Hirai, M. Bremholm, J. M. Allred, J. Krizan, L. M. Schoop, Q. Huang, J. Tao, and R. J. Cava, Phys. Rev. Lett. **110**, 166402 (2013), ISSN 00319007.

[2] S. G. Louie, K.-M. Ho, and M. L. Cohen, Phys. Rev. B **19**, 1774 (1979), URL `http://link.aps.org/doi/10.1103/PhysRevB.19.1774`.

[3] B. Meyer, C. Elsasser, and M. Fahnle, *FORTRAN90 Program for Mixed-Basis Pseudopotential Calculations for Crystals*.

[4] S. Baroni, S. de Gironcoli, A. Dal Corso, and P. Giannozzi, Rev. Mod. Phys. **73**, 515 (2001), URL `http://link.aps.org/doi/10.1103/RevModPhys.73.515`.

[5] R. Heid and K.-P. Bohnen, Phys. Rev. B **60**, R3709 (1999), URL `http://link.aps.org/doi/10.1103/PhysRevB.60.R3709`.

[6] D. Vanderbilt, Phys. Rev. B **32**, 8412 (1985), URL `http:`

//link.aps.org/doi/10.1103/PhysRevB.32.8412.

[7] L. Kleinman, Phys. Rev. B **21**, 2630 (1980), URL http://link.aps.org/doi/10.1103/PhysRevB.21.2630.

[8] G. B. Bachelet and M. Schlüter, Phys. Rev. B **25**, 2103 (1982), URL http://link.aps.org/doi/10.1103/PhysRevB.25.2103.

[9] R. Heid, K.-P. Bohnen, I. Y. Sklyadneva, and E. V. Chulkov, Phys. Rev. B **81**, 174527 (2010), URL http://link.aps.org/doi/10.1103/PhysRevB.81.174527.

[10] J. P. Perdew, K. Burke, and M. Ernzerhof, Phys. Rev. Lett. **77**, 3865 (1996), ISSN 1079-7114, URL http://www.ncbi.nlm.nih.gov/pubmed/10062328.

[11] C. L. Fu and K. M. Ho, Phys. Rev. B **28**, 5480 (1983), URL http://link.aps.org/doi/10.1103/PhysRevB.28.5480.
